# Supplementary material for: M2QA: Multi-domain Multilingual Question Answering
Source: arXiv:2407.01091 source file (2024-07-01)
Supplement: Supplementary file 1 [file appendix_eval_table.tex]

\begin{table*}[t]
    \centering
    \resizebox{\textwidth}{!}{%
    \begin{tabular}{lllcccccccccccccc}
        \toprule
         &   &   & \multicolumn{3}{c}{\textbf{Creative Writing}} & \multicolumn{3}{c}{\textbf{Product Reviews}}  & \multicolumn{3}{c}{\textbf{News}} & \multicolumn{5}{c}{\textbf{Average}}   \\
                    & &           & \multicolumn{2}{c}{answerable} & unansrbl& \multicolumn{2}{c}{answerable} & unansrbl& \multicolumn{2}{c}{answerable} & unansrbl& \multicolumn{2}{c}{answerable} & unansrbl & \multicolumn{2}{c}{Total Average}\\
         & Model      &           & F1    & EM & F1   & F1    & EM & F1    & F1    & EM & F1    & F1    & EM & F1    & F1 & EM\\
         \midrule
         \multirow{4}{*}{\rotatebox[origin=l]{90}{\textbf{German}}} & Llama 3-instruct (8b) &(0-shot) & \textbf{44.98}& \textbf{24.33}& 34.33& \textbf{45.19}& \textbf{24.56}& 32.17& \textbf{55.41}& 37.44& 30.33&       \textbf{48.53}&       \textbf{28.78}&   34.65&     42.98&   31.13\\   
         & Aya-23 (8B) &(0-shot)& 31.69& 19.89& 82.17& 35.82& 20.89& 81.67& 55.30& \textbf{39.78}& 74.00& 40.94& 26.85& 79.28& \textbf{56.28}& \textbf{47.82}\\
         \cmidrule(lr){2-3}\cmidrule(lr){4-6} \cmidrule(lr){7-9} \cmidrule(lr){10-12} \cmidrule(lr){13-17}
         & Llama 3-instruct (8b) &(5-shot) &    43.44&               23.89&              35.50&             39.82&     20.56&                  25.50&       54.71&        35.56&        28.00&       45.99&       26.67&   29.67&     39.46&   27.87\\
         & Aya-23 (8B) &(5-shot)& 16.44& 10.78& \textbf{90.83}& 19.85& 12.11& \textbf{93.67}& 38.00& 28.44& \textbf{89.33}& 24.76& 17.11&  \textbf{91.28}& 51.37&46.78\\
         
         \midrule
         \addlinespace
         \midrule
         \multirow{4}{*}{\rotatebox[origin=l]{90}{\textbf{Turkish}}}& Llama 3-instruct (8b) &(0-shot) & 46.27& 31.67& 25.17& 54.06& 28.56& 36.50& 53.91& 32.67& 26.50&       51.41&       30.97&   29.39&     59.35&   30.34\\   
         & Aya-23 (8B) &(0-shot)& 41.74& 31.11& 65.83& 52.93& 30.78& 59.83& 52.59& 32.56& 54.33& 49.09& 31.48& 60.00& 53.45& 42.89\\
         \cmidrule(lr){2-3}\cmidrule(lr){4-6} \cmidrule(lr){7-9} \cmidrule(lr){10-12} \cmidrule(lr){13-17}
         & Llama 3-instruct (8b) &(5-shot) &    38.73&               24.33&              47.33&             41.27&     21.89&                  42.33&       51.15&        30.22&        25.83&       43.72&       25.48&   38.50&     41.63&   30.69\\
         & Aya-23 (8B) &(5-shot)& 28.52& 21.89& 79.33& 33.14& 20.56& 84.67& 32.95& 20.44& 74.00& 31.54& 20.96&  79.33& 50.66&44.31\\
         
         \midrule
         \addlinespace
         \midrule

         \multirow{4}{*}{\rotatebox[origin=l]{90}{\textbf{Chinese}}} & Llama 3-instruct (8b) &(0-shot) & \textbf{36.61}& 33.33& 29.17& 27.52& 23.33& 32.17& 33.50& 21.00& 26.83&       32.54&       25.89&   29.39&     31.28&   27.29\\   
         & Aya-23 (8B) &(0-shot)& 35.44& \textbf{35.44}& 56.83& 26.74& 26.74& 65.33& 50.39& 33.67& 47.33& 37.52& 31.95& 56.50& 45.11& 41.77\\
         \cmidrule(lr){2-3}\cmidrule(lr){4-6} \cmidrule(lr){7-9} \cmidrule(lr){10-12} \cmidrule(lr){13-17}
         & Llama 3-instruct (8b) &(5-shot) &    34.78&               32.22&              34.83&             21.16&     17.67&                  32.67&       33.21&        20.67&        22.83&       29.72&       23.52&   30.11&     29.88&   26.16\\
         & Aya-23 (8B) &(5-shot)& 28.11& 28.11& 60.33& 22.74& 22.67& 61.17& 50.40& 34.33& 50.83& 33.75& 28.37&  57.44& 43.23&40.00\\

         \bottomrule

    \end{tabular}
    }
    % \vspace{-2mm}
    \caption{TODO   }
    % \vspace{-4.5mm}
    \label{tab:appendix_additional_llm_results}
\end{table*}
